# Supplementary material for: GRIN: GRadient-INformed MoE
Source: arXiv:2409.12136 source file (2024-09-18)
Supplement: Supplementary file 1 [file 5a-inference-appendix.tex]

%\begin{figure}
%    \centering
%    \vspace{-10pt}
%    \begin{minipage}[b]{0.45\textwidth}
%        \centering
%        \includegraphics[width=1\linewidth]{figure/inference-breakdown-p2048d1024.png}
%        \label{fig:infer_p2048d1024}
%    \end{minipage}
%    \hfill
%    \begin{minipage}[b]{0.45\textwidth}
%        \centering
%        \includegraphics[width=1\linewidth]{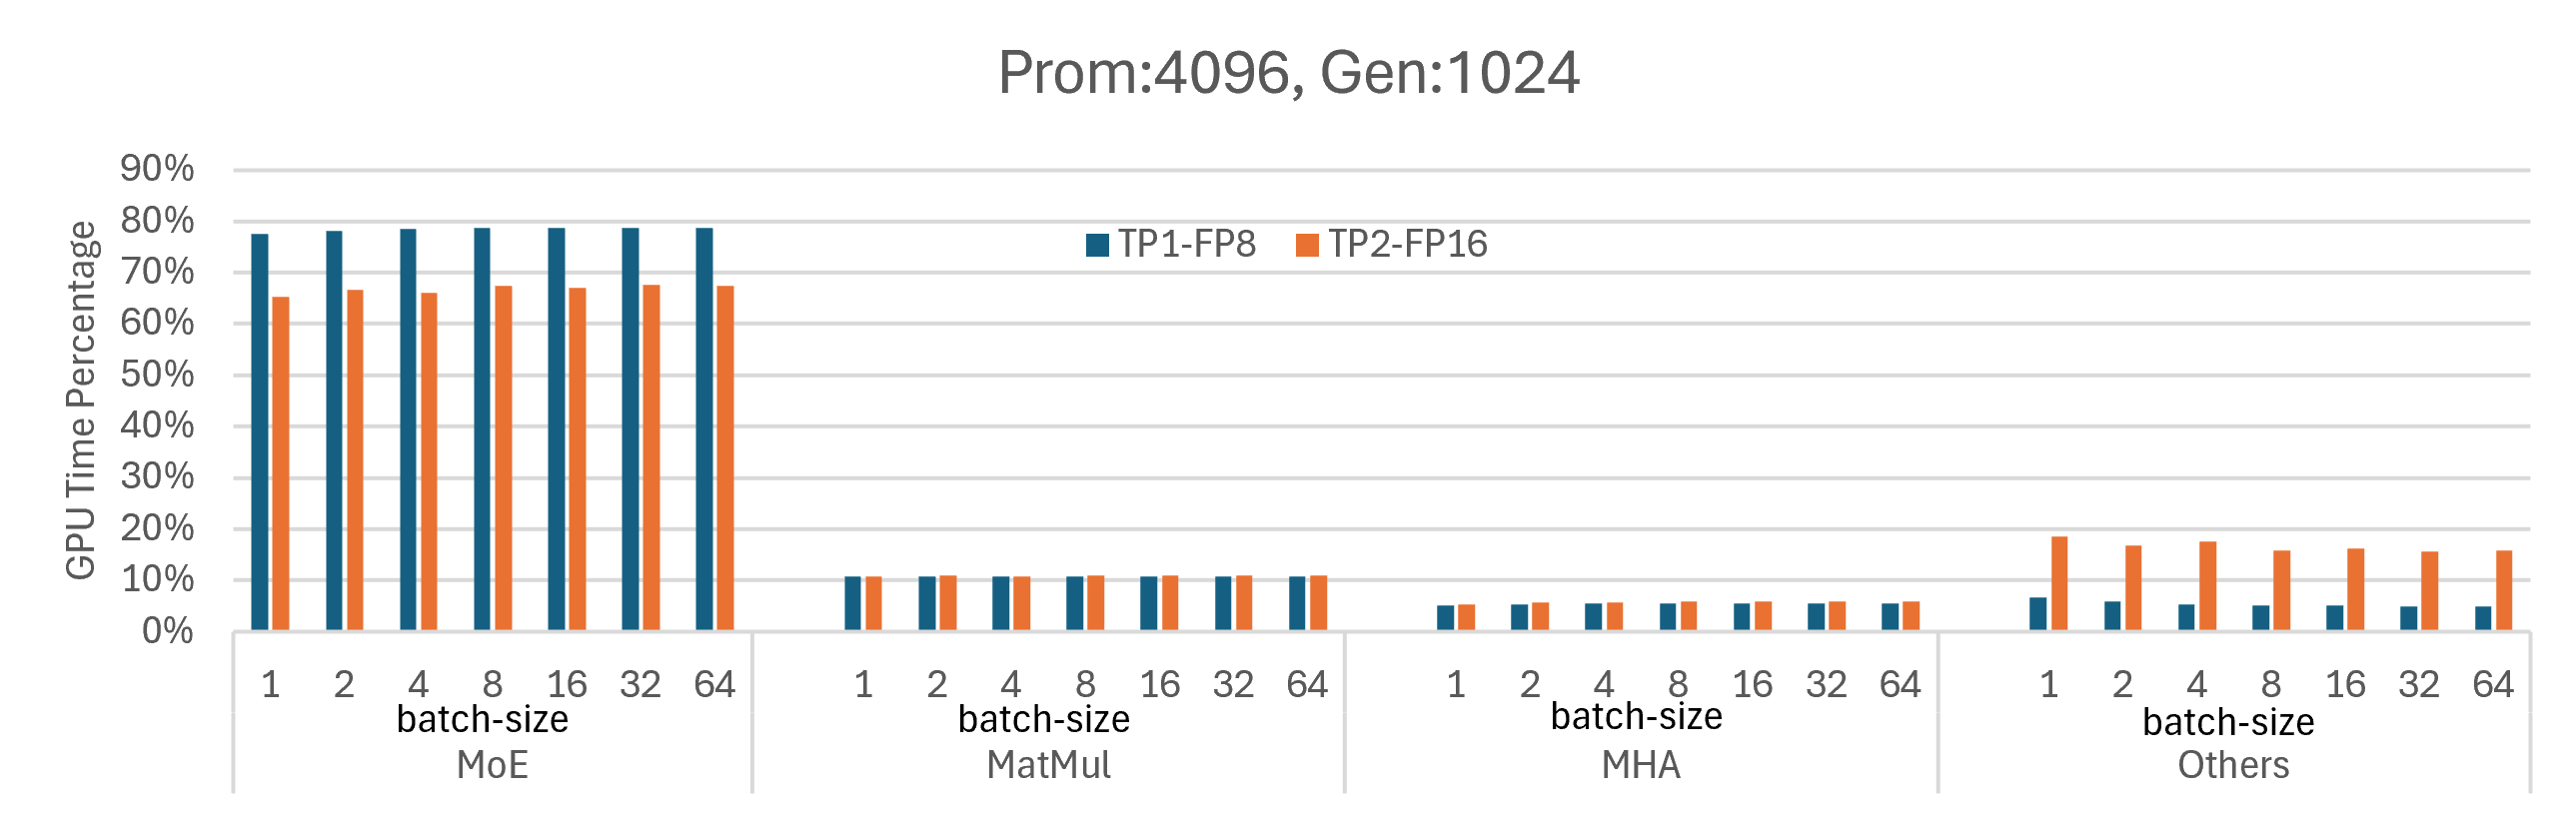}
%        \label{fig:infer_p2048d1024}
%    \end{minipage}
%\end{figure}
\section{Model Inference Breakdown}\label{appendix:inference}
The inference efficiency of \ourmodel is further analyzed in Figure~\ref{fig:inference-breakdown} and Figure~\ref{fig:inference-breakdown-ratio}. 

\begin{figure}[h]
    \centering
    % \vspace{-10pt}
        \includegraphics[width=1.\linewidth]{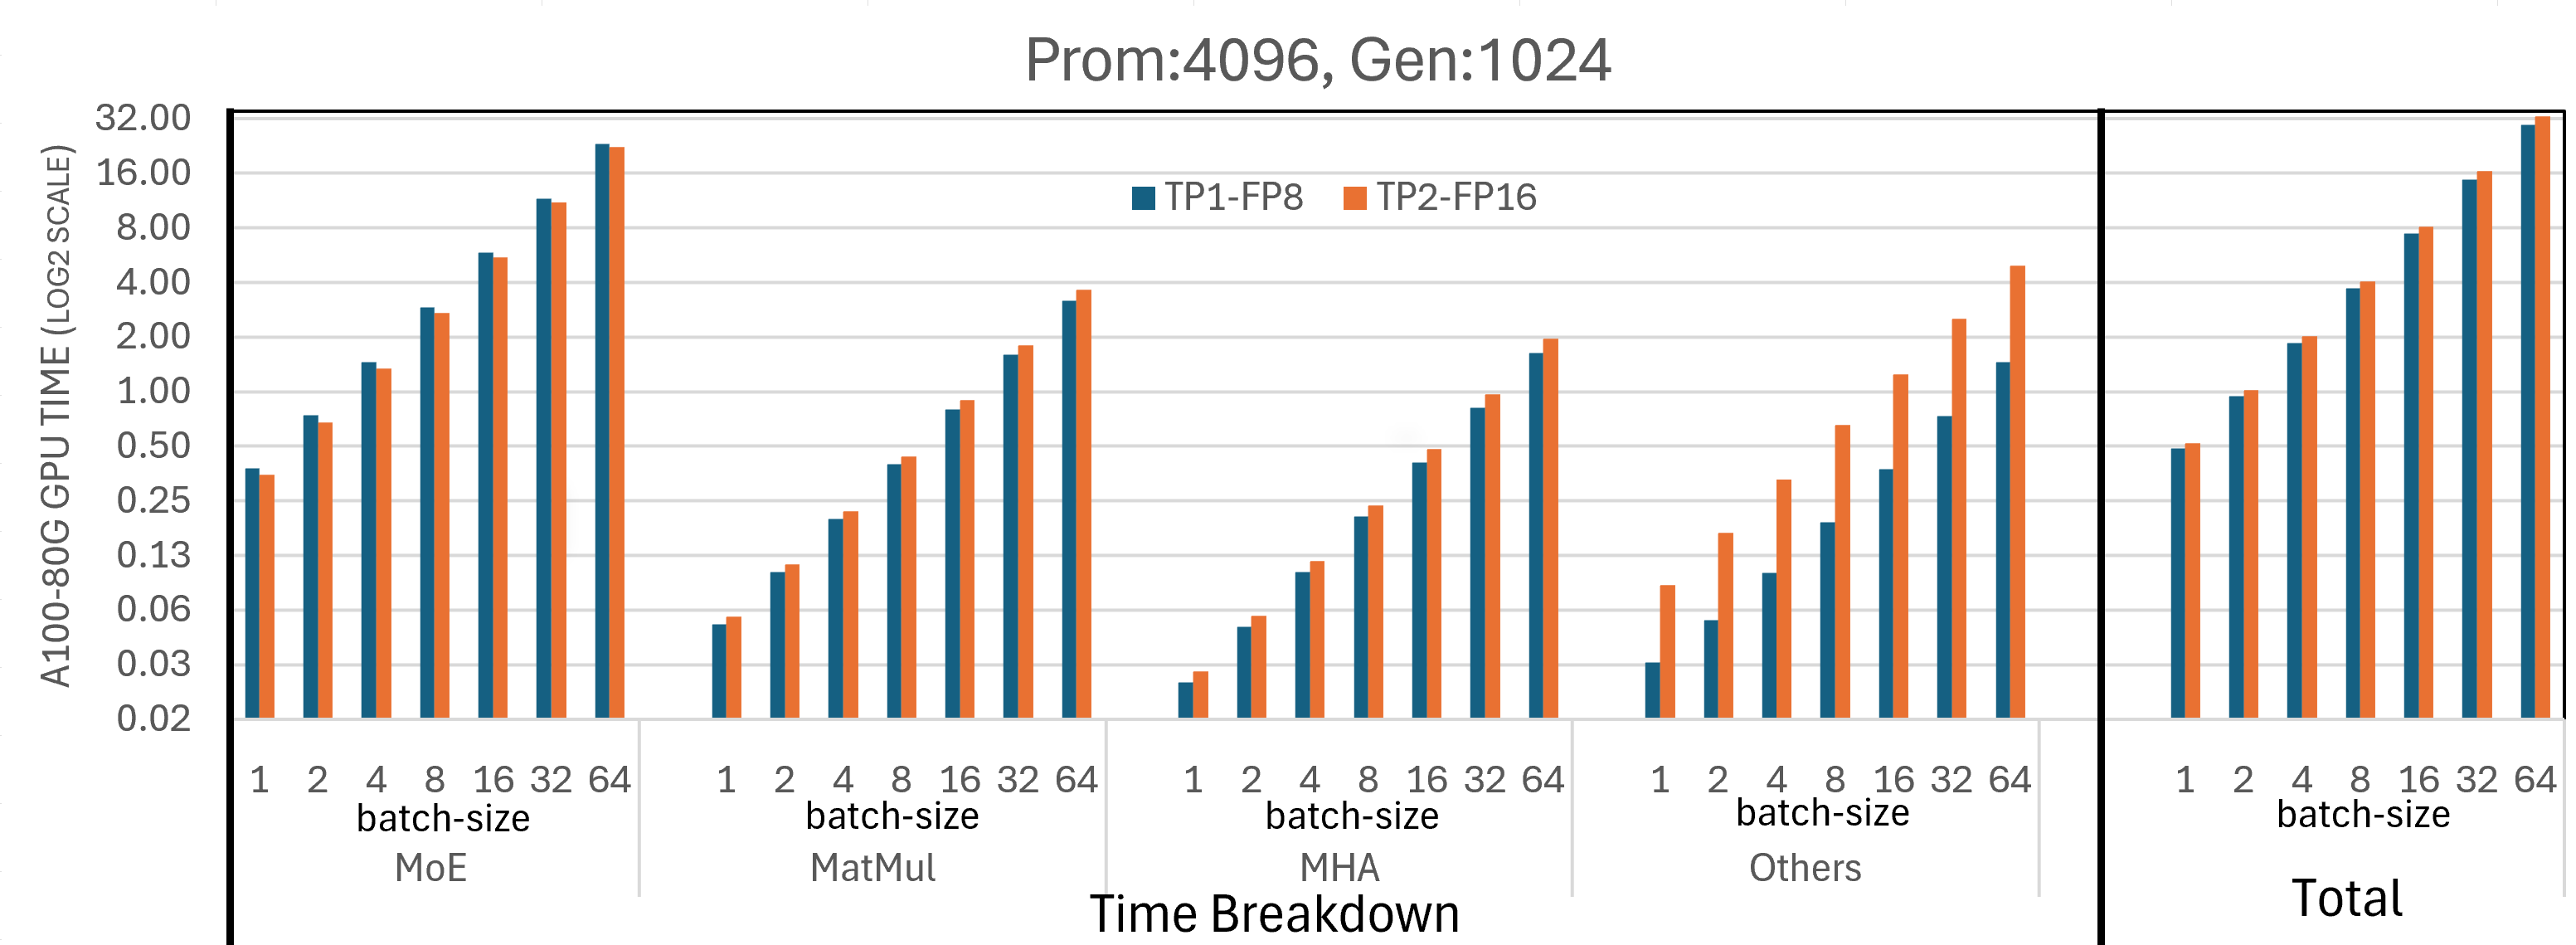}
    \caption{\ourmodel inference at different batch sizes. MatMul: matrix multiplication for dense layers, which includes all MatMul kernels not involved with MHA or MoE;
MHA: multi-head attention; MoE: expert layers, which includes SparseMixer kernels, data movement kernels, activation kernels and MatMul kernels within MoE; Others: including other GPU kernels or GPU idle time or NCCL time if applicable.The GPU time is measured by second.}
    \label{fig:inference-breakdown}
\end{figure}
\begin{figure}[h]
    \centering
    % \vspace{-10pt}
        \includegraphics[width=1.\linewidth]{figure/inference-breakdown-p4096d1024.png}
    \caption{\ourmodel inference kernels latency percentage at different batch sizes. Categories MatMul, MHA, MoE, Others are as same as Figure \ref{fig:inference-breakdown}}
    \label{fig:inference-breakdown-ratio}
\end{figure}
